# Supplementary material for: Information Bottleneck Revisited: Posterior Probability Perspective with Optimal Transport
Source: arXiv:2308.11296 source file (2023-08-22)
Supplement: Supplementary file 1 [file appendix.tex]

\begin{appendix} \label{ap_AS_detail}
For convenience, we restate the Lagrangian of the IB-OT model \eqref{Lagrangian_used} as follows
\begin{small}
\begin{equation*} \label{Lagrangian}
\begin{aligned}
&\mathcal{L}(\bdw,\bdr,\bdz; \bda, \bdb, \bm{\lambda}, {\eta},\zeta)=\sum_{i=1}^{M} \sum_{j=1}^{N} w_{i j}r_j\log w_{i j} \\
&+ \sum_{i=1}^{M} \alpha_{i} \bigg(\sum_{j=1}^{N} w_{i j}r_j-p_i\bigg)+\sum_{j=1}^{N}\beta_{j}\bigg(\sum_{i=1}^{M} w_{i j} r_j-r_{j}\bigg) \\
&+\sum_{j=1}^N\sum_{k=1}^K{\lambda_{kj}}\bigg(\sum_{i=1}^{M}w_{ij}r_j s_{ki}-z_{kj}\bigg) + {\eta}\bigg(\sum_{j=1}^{N} r_{j}-1\bigg)\\
&-\zeta \bigg( \sum_{j=1}^N\sum_{k=1}^K \Big(\sum_{i=1}^{M}w_{ij}s_{ki}r_j\Big)\log z_{kj}\!\!-\!\!\sum_{j=1}^N r_{j}\log r_{j} \!\!-\!\! \hat{I} \bigg).
\end{aligned}
\end{equation*}
\end{small}
We update the variables $\bdw,\bdz,\bdr$ as well as the associated dual variables $\bda,\bdb,\bdlam,$ in the following manner.

\subsection{Updating the variable $\bdw$ and its dual variables}

Taking the derivative of $\mathcal{L}(\bdw, \bdr,\bdz; \bda, \bdb, \bm{\lambda}, {\eta},\zeta)$ with respect to the primal variable $\bdw$, one obtains
\begin{equation*} \label{dW}
\begin{aligned}
    \frac{\partial \mathcal{L}}{\partial w_{i j}}=r_j(1+\log w_{i j})+\alpha_{i}r_j+\beta_{j}r_j \\
    +\sum_{k=1}^{K} \lambda_{k j} s_{k i} r_j-\zeta \sum_{k=1}^K s_{ki}r_j\log z_{kj},
\end{aligned}
\end{equation*}
and it further yields the representation of $\bdw$ by dual variables
\begin{equation} \label{update_W}
w_{i j}=\exp \left(-\alpha_{i}-1 / 2\right)  \Lambda_{ij} \exp \left(-\beta_{j}-1 / 2\right).
\end{equation}
Here, denote $\phi_{i}=\exp\left(-{\alpha_{i}}-{1}/{2}\right)$, $\psi_{j}=\exp\left(-\beta_{j}-{1}/{2}\right)$ and $\Lambda_{ij}=\exp \left(-\sum_{k=1}^{K} s_{k i}(\lambda_{k j} -\zeta \log z_{kj})\right)$ for simplicity, then \eqref{update_W} yields
\begin{equation*}
w_{ij}=\phi_{i}\Lambda_{ij}\psi_{j}.
\end{equation*}
Substituting the above formula into \eqref{IB_OT_model_b}, we get
\begin{subequations} \label{ot_cont}
\begin{align} 
&\phi_{i} \sum_{j=1}^{N} \Lambda_{ij} \psi_{j} r_{j}=p_i, \quad i=1, \cdots, M, \label{ot_cont_a} \\
&\psi_{j} r_{j} \sum_{i=1}^{M} \Lambda_{ij} \phi_{i}=r_{j}, \quad j=1, \cdots, N. \label{ot_cont_b}
\end{align}
\end{subequations}
By eliminating $r_{j}$ on both side of the \eqref{ot_cont_b}, we can alternatively update $\psi_{j}$ and $\phi_{i}$ by the Sinkhorn algorithm as follows,
\begin{equation}\label{ot_sinkhorn} 
\psi_{j} = 1 \Big/ \sum_{i=1}^{M} \Lambda_{ij} \phi_{i} , \quad \phi_{i} = p_i \Big/ \sum_{j=1}^{N} \Lambda_{ij} \psi_{j} r_{j}.
\end{equation}
Next, taking the derivative of $\mathcal{L}\left({\bdw}, \bdr, \bdz; \bda, \bdb, \bm{\lambda}, \eta,\zeta\right)$ with respect to $\zeta$, we have the following condition for $\zeta\in\mbbR^{+}$,
\begin{small}
\begin{multline*}\label{G_def}
    G(\zeta) \triangleq-\Big(\sum_{j=1}^{N} r_{j} \log r_{j}+\hat{I}\Big)+\sum_{j,k=1}^{N,K}\bigg(\sum_{i=1}^{M}\phi_is_{ki} \\
    \times\exp\Big(-\sum_{k'=1}^{K} s_{k'i}(\lambda_{k'j}-\zeta \log z_{k'j})\Big)\bigg)\psi_jr_j\log z_{kj}=0.
\end{multline*}
\end{small}
Note that the derivative of $G(\zeta)$ is positive, due to $\log z_{kj}<0$, \thatis,
\begin{small}
\begin{equation*}
\begin{aligned}
    G^{\prime}(\zeta)= &\sum_{j,k=1}^{N,K} \bigg( \sum_{i=1}^{M} \phi_i\exp\Big(-\sum_{k=1}^K s_{ki}(\lambda_{kj}-\zeta \log z_{kj})\Big)\\
    &\times \Big(\sum_{k=1}^K s_{ki}\log z_{kj}\Big)\psi_j s_{k i}r_j \bigg)\log z_{k j}>0,
\end{aligned}
\end{equation*}
\end{small}
and then $G(\zeta)$ is monotonic.
Therefore, we are able to update $\zeta(\ge 0)$ by finding the root of $G(\zeta)$ with Newton's method.
Moreover, we need to discuss the feasibility of the Sinkhorn iteration, especially \textcolor{black}{under} the extra constraint \eqref{IB_OT_model_d}. Depending on the value of $G(0)$, there are two cases:
\begin{itemize}
    \item $G(0)<0$: In this case, $G(\zeta)=0$ has a unique solution on $(0,+\infty)$ since $G'(\zeta)>0$. Thus the extra constraint \eqref{IB_OT_model_d} is obviously satisfied.
    
    \item $G(0)\geq 0$: In this case, the extra constraint \eqref{IB_OT_model_d} is already satisfied. We only need to set $\zeta=0$ instead of solving $G(\zeta)=0$ at line 6 of Algorithm \ref{alg:OT_ibp}.
\end{itemize}

\subsection{Updating the variable $\bdz$ and its dual variables}

Taking the derivative of $\mathcal{L}(\bdw, \bdr,\bdz; \bda, \bdb, \bm{\lambda}, {\eta},\zeta)$ with respect to the primal variable $\bdz$ derives the following equation
\begin{equation}
\frac{\partial \mathcal{L}}{\partial z_{k j}}=-\lambda_{k j}-\zeta\frac{\left(\sum_{i=1}^{M} s_{ki}w_{ij}r_j\right)}{z_{kj}},
\end{equation}
which yields a representation of $\bdz$ by dual variables $\zeta,\bm{\lambda}$, \thatis,
\begin{equation}\label{from_of_z}
z_{kj} = -\zeta\left(\sum_{i=1}^{M} s_{ki}w_{ij}r_j\right)\bigg/\lambda_{kj}.
\end{equation}
Substituting \eqref{from_of_z} into the constraint $\sum_{i=1}^{M}w_{ij}r_j s_{ki}=z_{kj}$ in \eqref{IB_OT_model_c}, we figure out the dual variable $\bm{\lambda}$ as follows,
\begin{equation}
\lambda_{kj}=-\zeta. \label{F_def}
\end{equation}

\subsection{Updating the variable $\bdr$ and its dual variables}

Taking the derivative of $\mathcal{L}(\bdw, \bdr,\bdz; \bda, \bdb, \bm{\lambda}, {\eta},\zeta)$ with respect to the primal variable $\bdr$ derives the following equation
$$
\begin{aligned}
&\frac{\partial \mathcal{L}}{\partial r_{j}}=\zeta\left(1+\log r_{j}\right)-\beta_{j}+\sum_{i=1}^M w_{ij}\log w_{ij}\\
&-\zeta \sum_{i=1}^M\sum_{k=1}^K s_{ki}w_{ij}\log z_{kj} \\
&+\sum_{i=1}^M \alpha_i w_{ij}+\sum_{i=1}^M \beta_j w_{ij}+\sum_{i=1}^M\sum_{k=1}^K s_{ki}w_{ij}\lambda_{kj}+\eta,
\end{aligned}$$
which yields a representation of $\bdr$ by dual variables $\eta$, \thatis,
\begin{small}
\begin{equation}\label{from_of_r}
\begin{aligned}
    &r_{j}=\exp \bigg(\!-\frac{1}{\zeta}\Big(\sum_{i=1}^M w_{ij}\log w_{ij}\!-\!\zeta \sum_{i=1}^M\sum_{k=1}^K s_{ki}w_{ij}\log z_{kj}\\
    &\!+\!\sum_{i=1}^M \alpha_i w_{ij}\!+\!\sum_{i=1}^M \beta_j w_{ij}\!+\!\sum_{i=1}^M\sum_{k=1}^K s_{ki}w_{ij}\lambda_{kj}\!-\!\beta_{j}\!+\!\eta\Big)\!-\!1\bigg).\\
\end{aligned}
\end{equation}
\end{small}
Substituting \eqref{from_of_r} into the equality constraint $\sum_{j=1}^N r_j =1$ in  \eqref{IB_OT_model_c}, we have the following equation
\begin{small}
\begin{equation*}
\begin{aligned}
    &\sum_{j=1}^N\exp \bigg(-\frac{1}{\zeta}\Big(\sum_{i=1}^M w_{ij}\log w_{ij}-\zeta \sum_{i=1}^M\sum_{k=1}^K s_{ki}w_{ij}\log z_{kj}-\!\beta_{j}\!\\
&\!+\!\sum_{i=1}^M \alpha_i w_{ij}\!+\!\sum_{i=1}^M \beta_j w_{ij}\!+\!\sum_{i=1}^M\sum_{k=1}^K s_{ki}w_{ij}\lambda_{kj}\!+\!\eta\Big)\!-\!1\bigg)=1.
\end{aligned}
\end{equation*}
\end{small}
We can update $\eta$ from this equation, and then we substitute it into \eqref{from_of_r}. We will get an explicit representation of $\bdr$, \thatis,
\begin{small}
\begin{equation*}
\begin{aligned}
&\tilde{r_{j}}=\exp \bigg(-\frac{1}{\zeta}\Big(\sum_{i=1}^M w_{ij}\log w_{ij}-\zeta \sum_{i=1}^M\sum_{k=1}^K s_{ki}w_{ij}\log z_{kj}\\
&\!+\!\sum_{i=1}^M \alpha_i w_{ij}\!+\!\sum_{i=1}^M \beta_j w_{ij}\!+\!\sum_{i=1}^M\sum_{k=1}^K s_{ki}w_{ij}\lambda_{kj}\!-\!\beta_{j}\!\Big)\!-\!1\bigg), \\
& r_j=\tilde{r_{j}}\Big/\Big(\sum_{j=1}^N \tilde{r_{j}}\Big). 
\end{aligned}
\end{equation*}
\end{small}

\end{appendix}
